# Supplementary material for: Patch-Based Image Inpainting with Generative Adversarial Networks
Source: arXiv:1803.07422 source file (2018-03-20)

# Supplementary Materials: Patch-Based Image Inpainting with Generative Adversarial Networks

## 1. Additional visual results

Following figures show the visual results obtained by the proposed PGGAN algorithm. Input images are taken from ImageNet[1], Google Street View[2] and Places2[3] datasets.

### 1.1. ImageNet

We perform high resolution inpainting experiments on ImageNet dataset. Input images are scaled to 512x512 and randomly located regions are cropped. Our model can successfully fill the blank areas as demonstrated in following figures.

Input Output

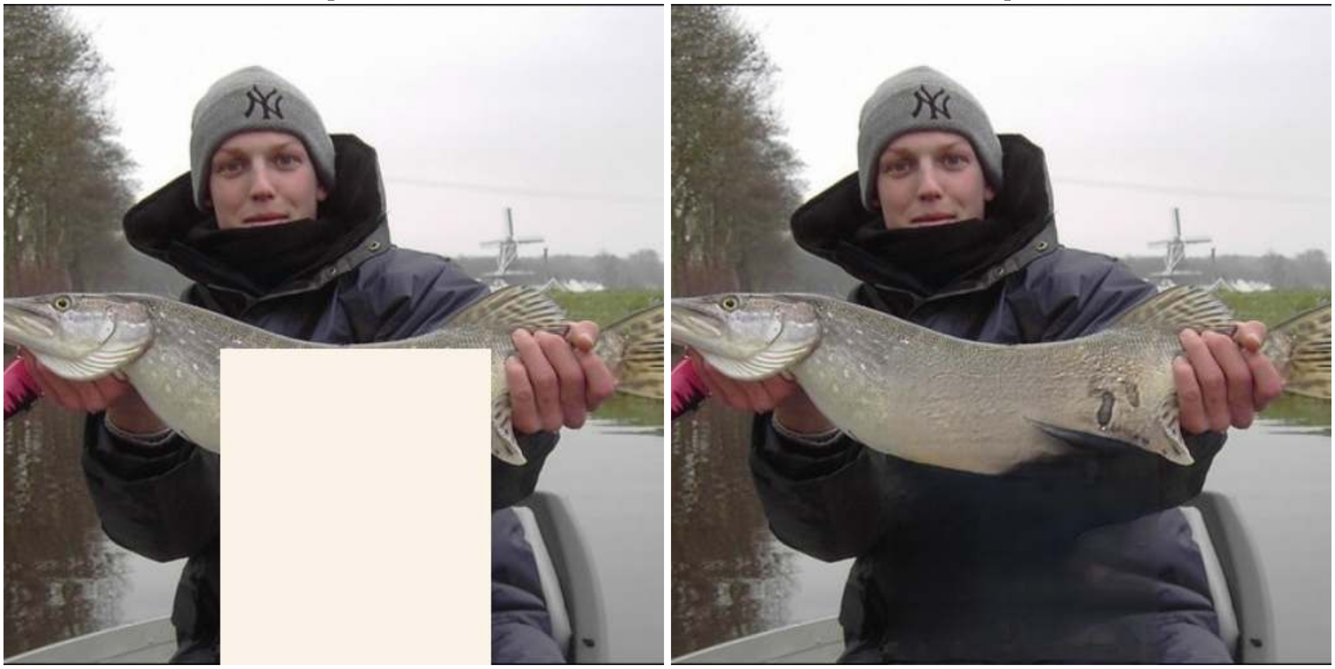

[1]http://image-net.org
[2]http://crcv.ucf.edu/data/GMCP_Geolocalization
[3]http://places2.csail.mit.edu

Input Output

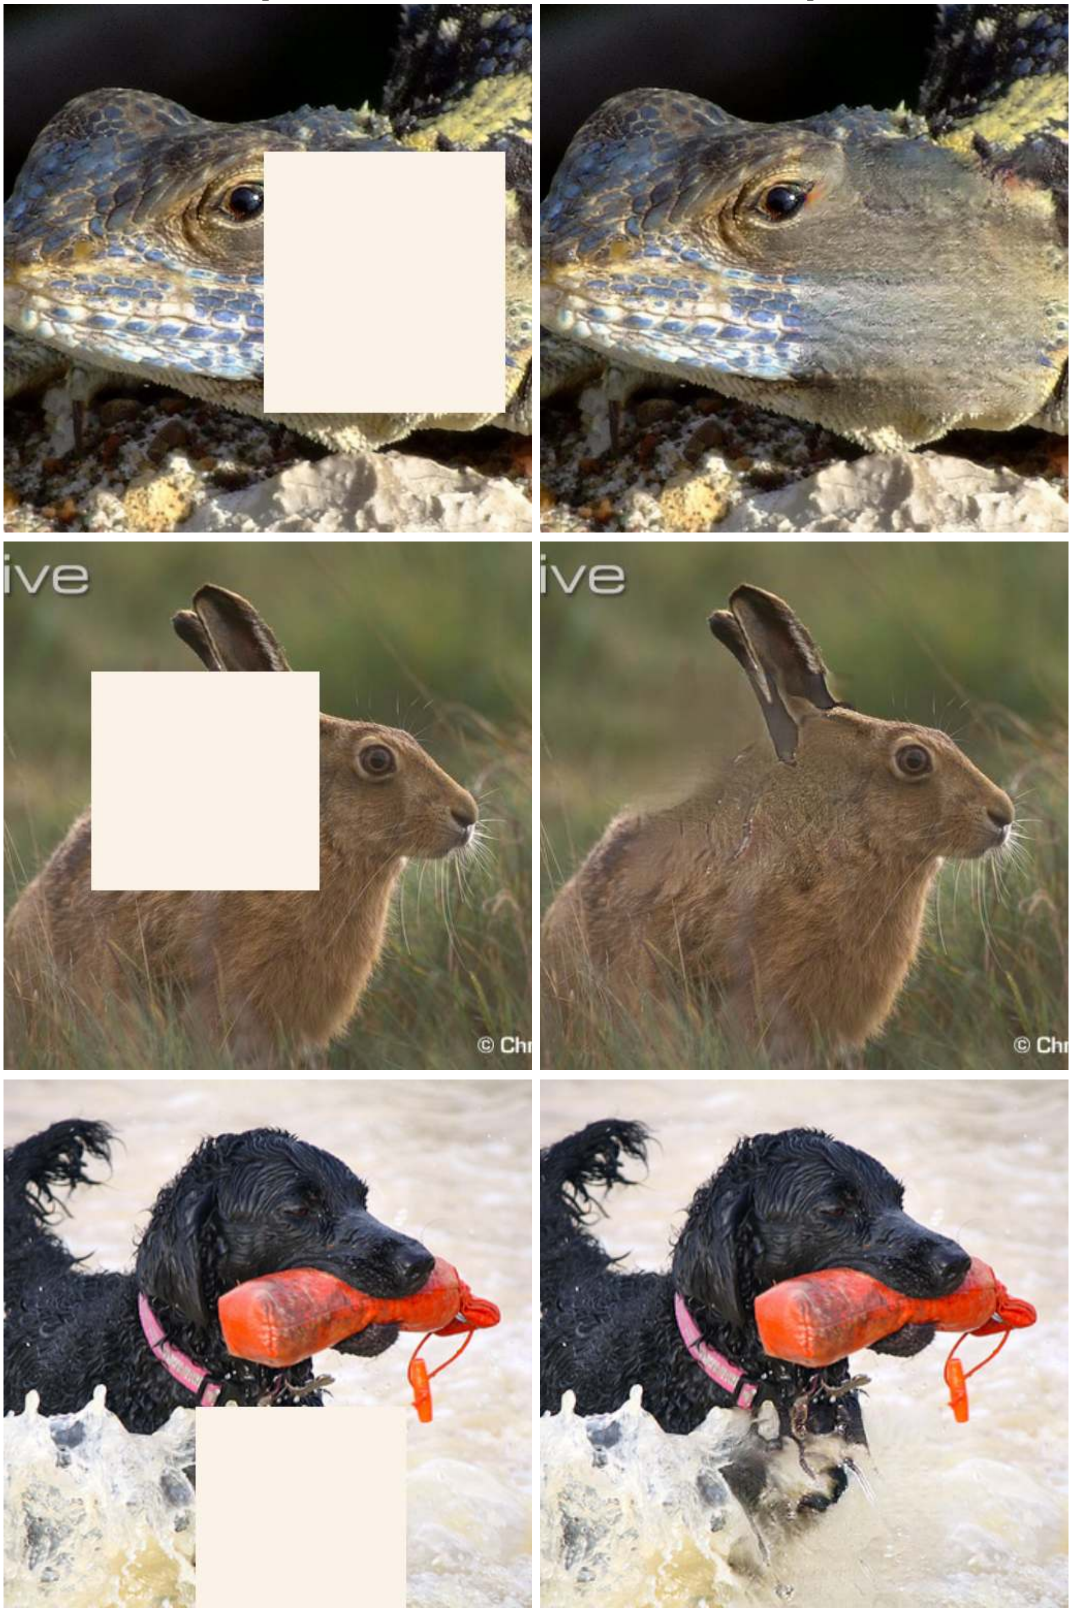

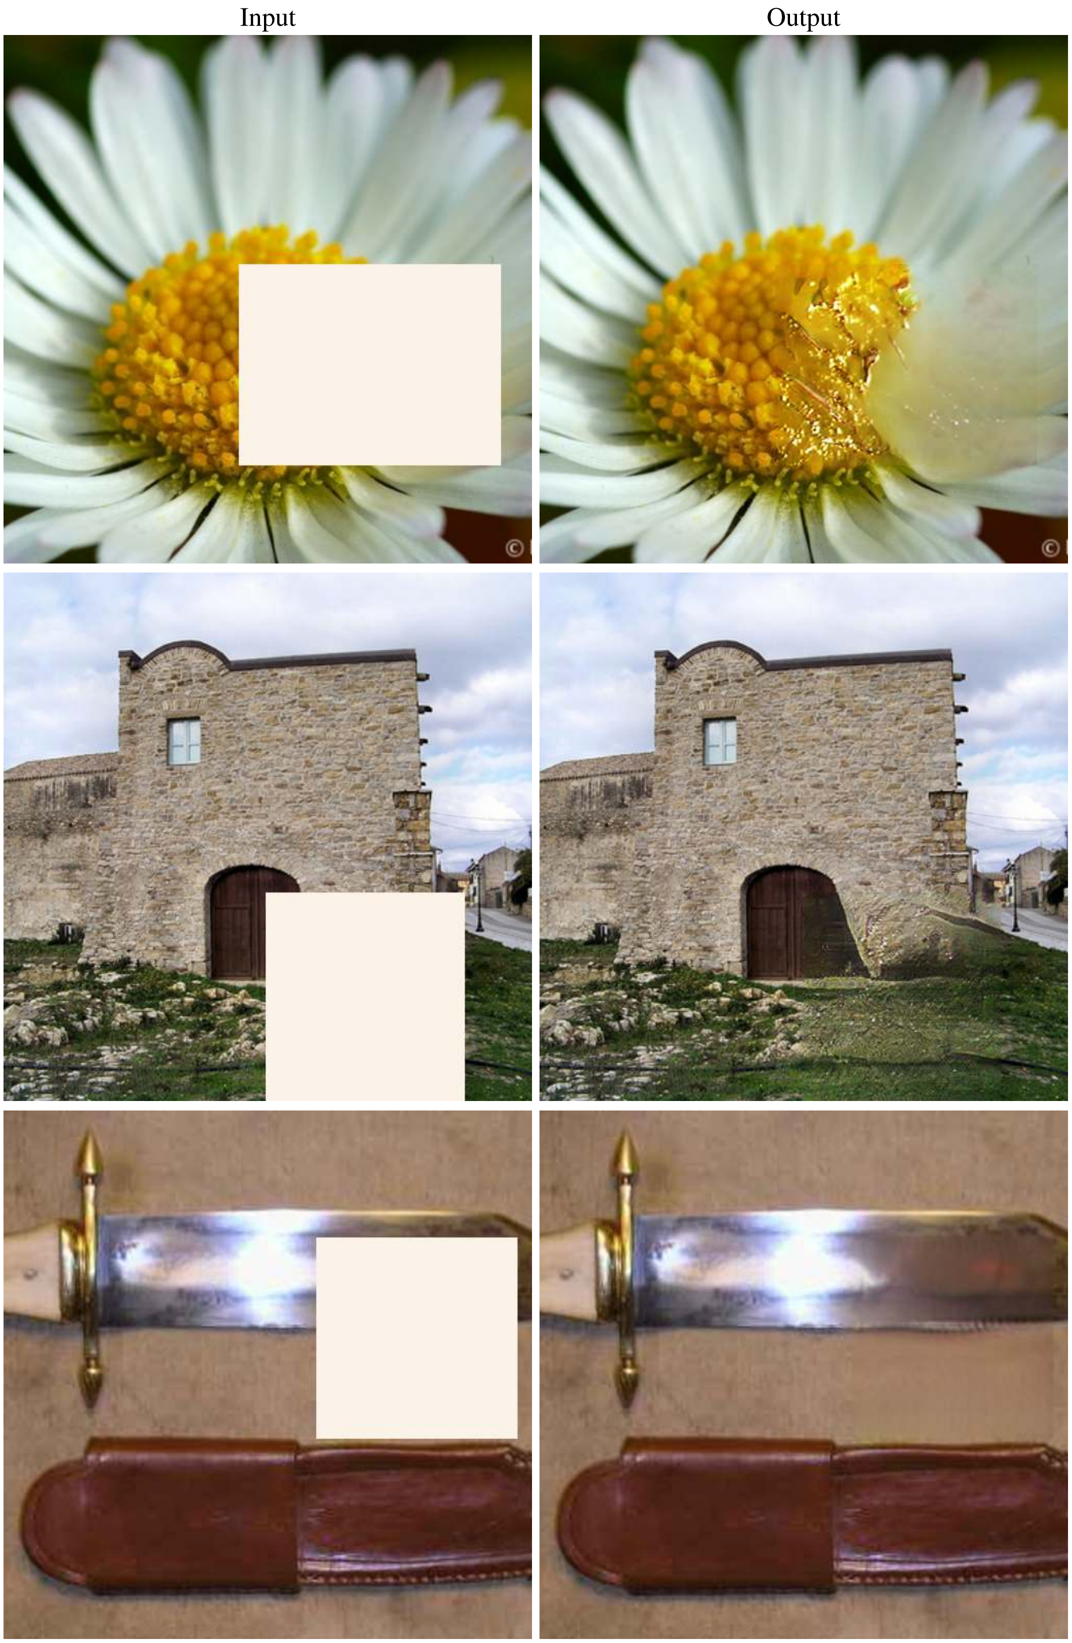
Input
Output

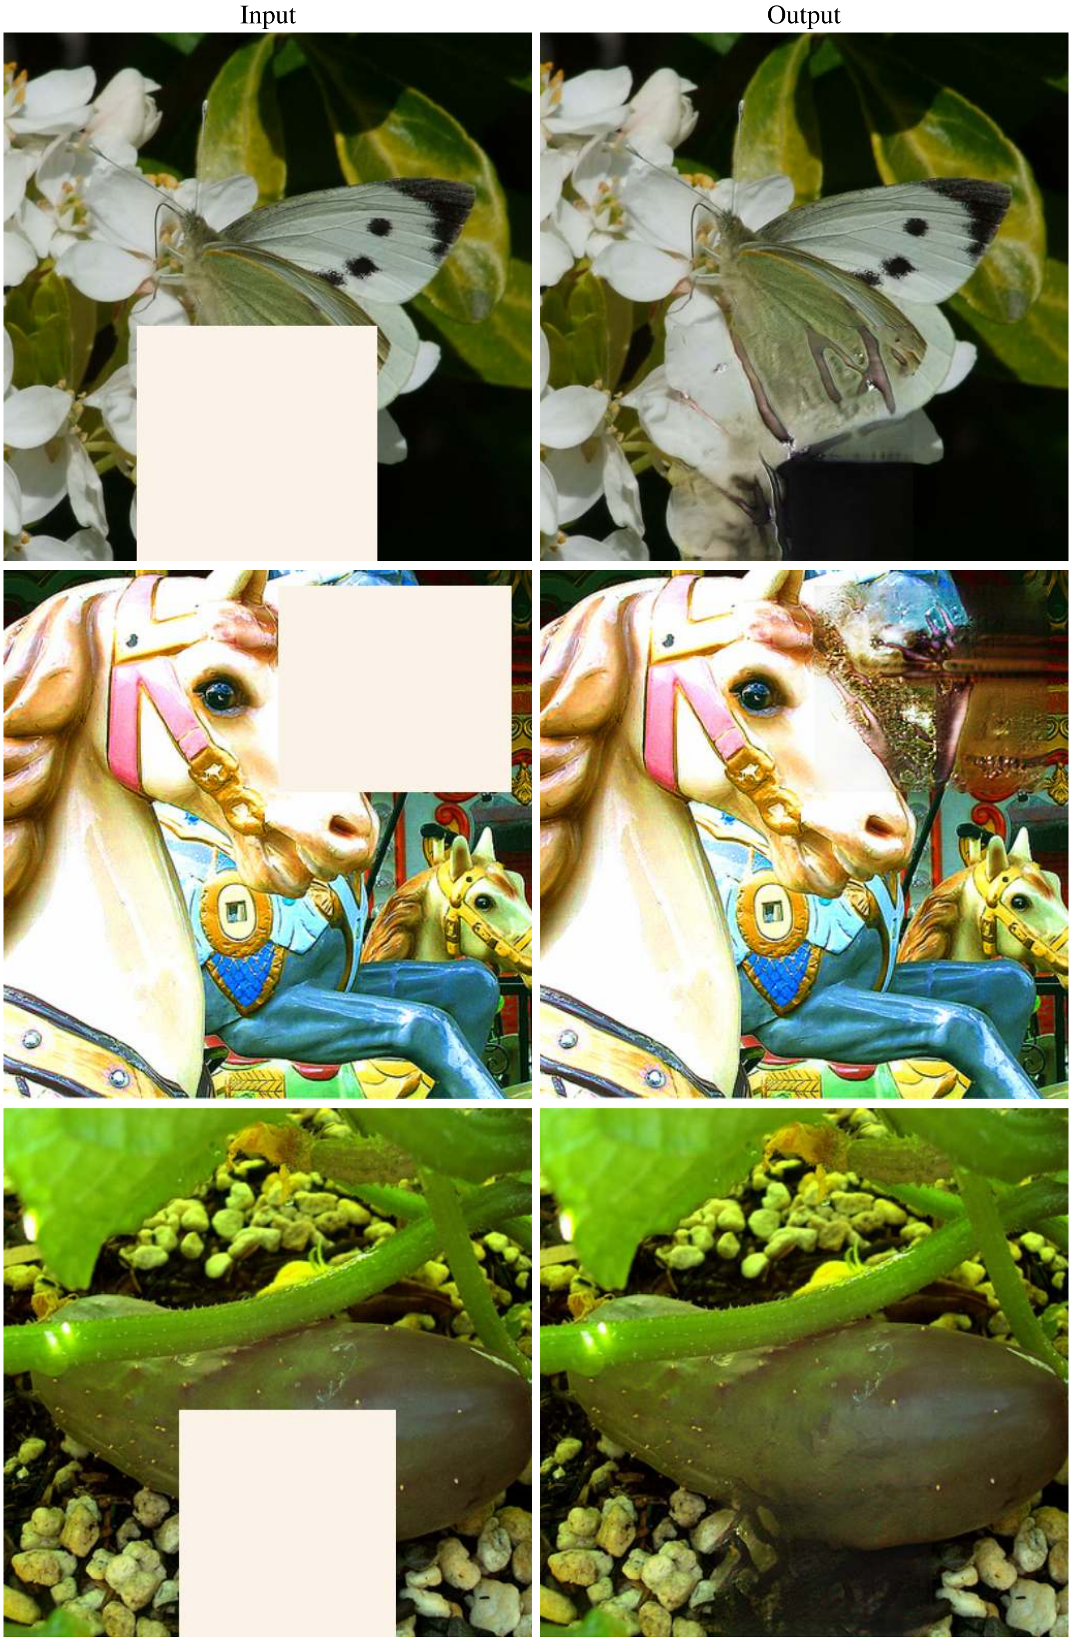
Input
Output

Input Output

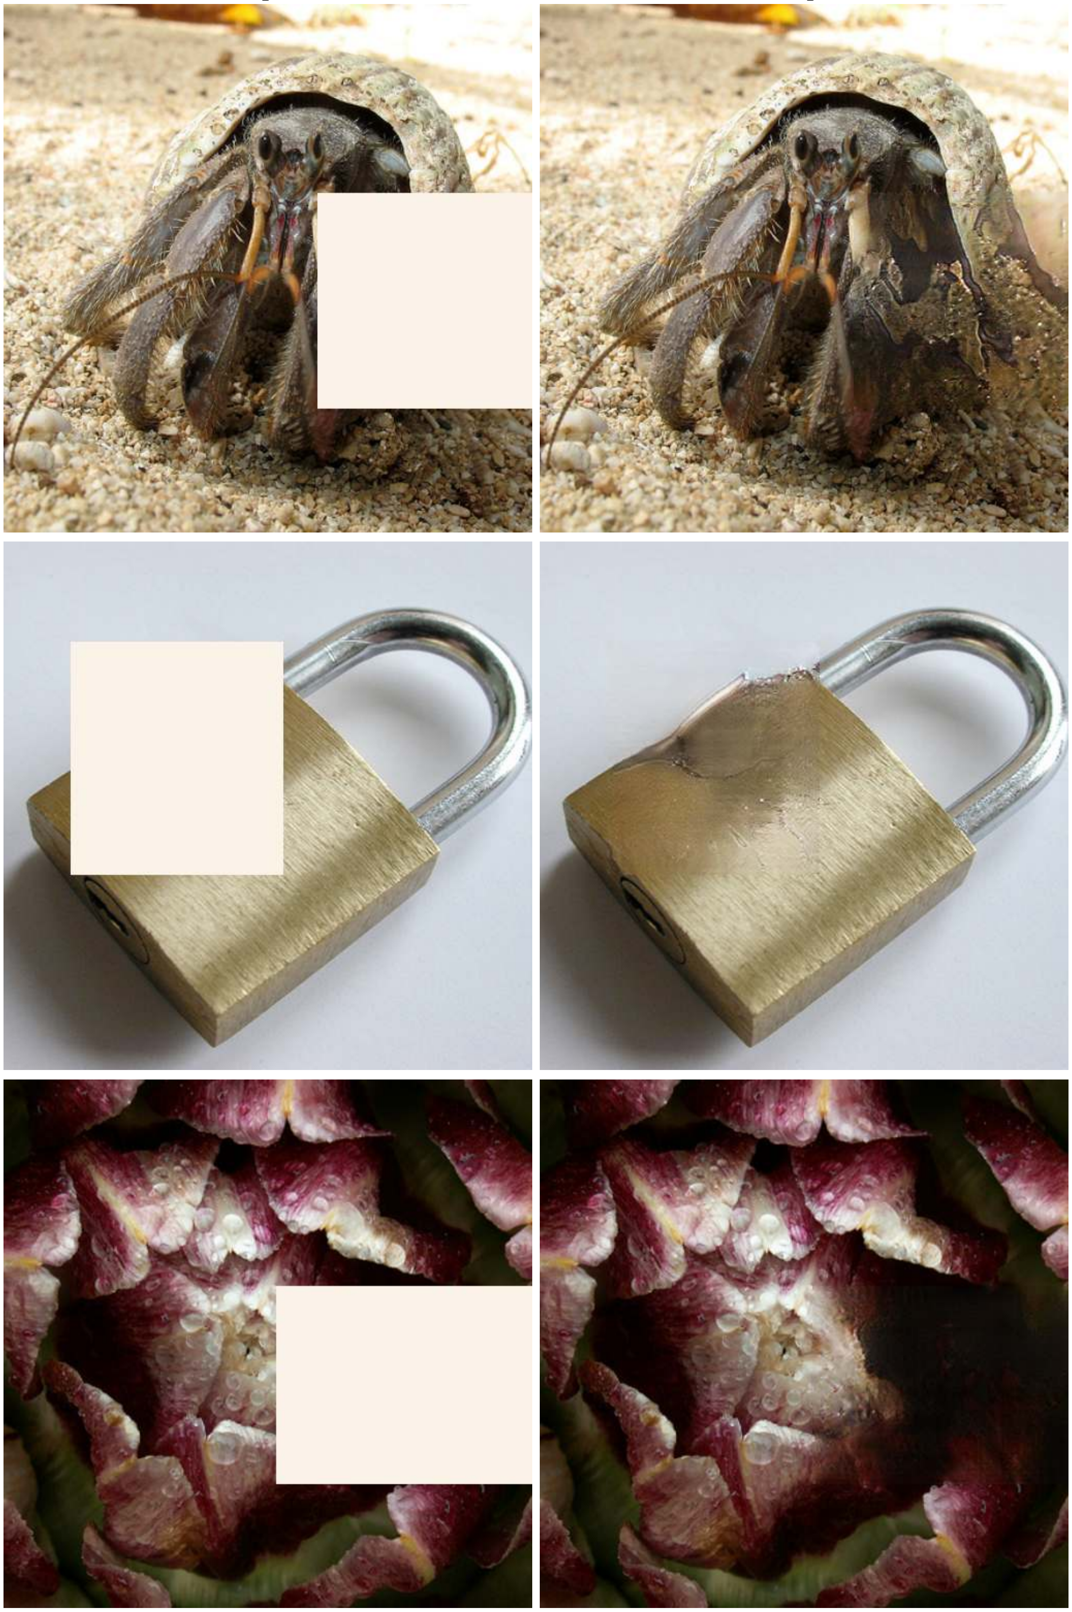

Input Output

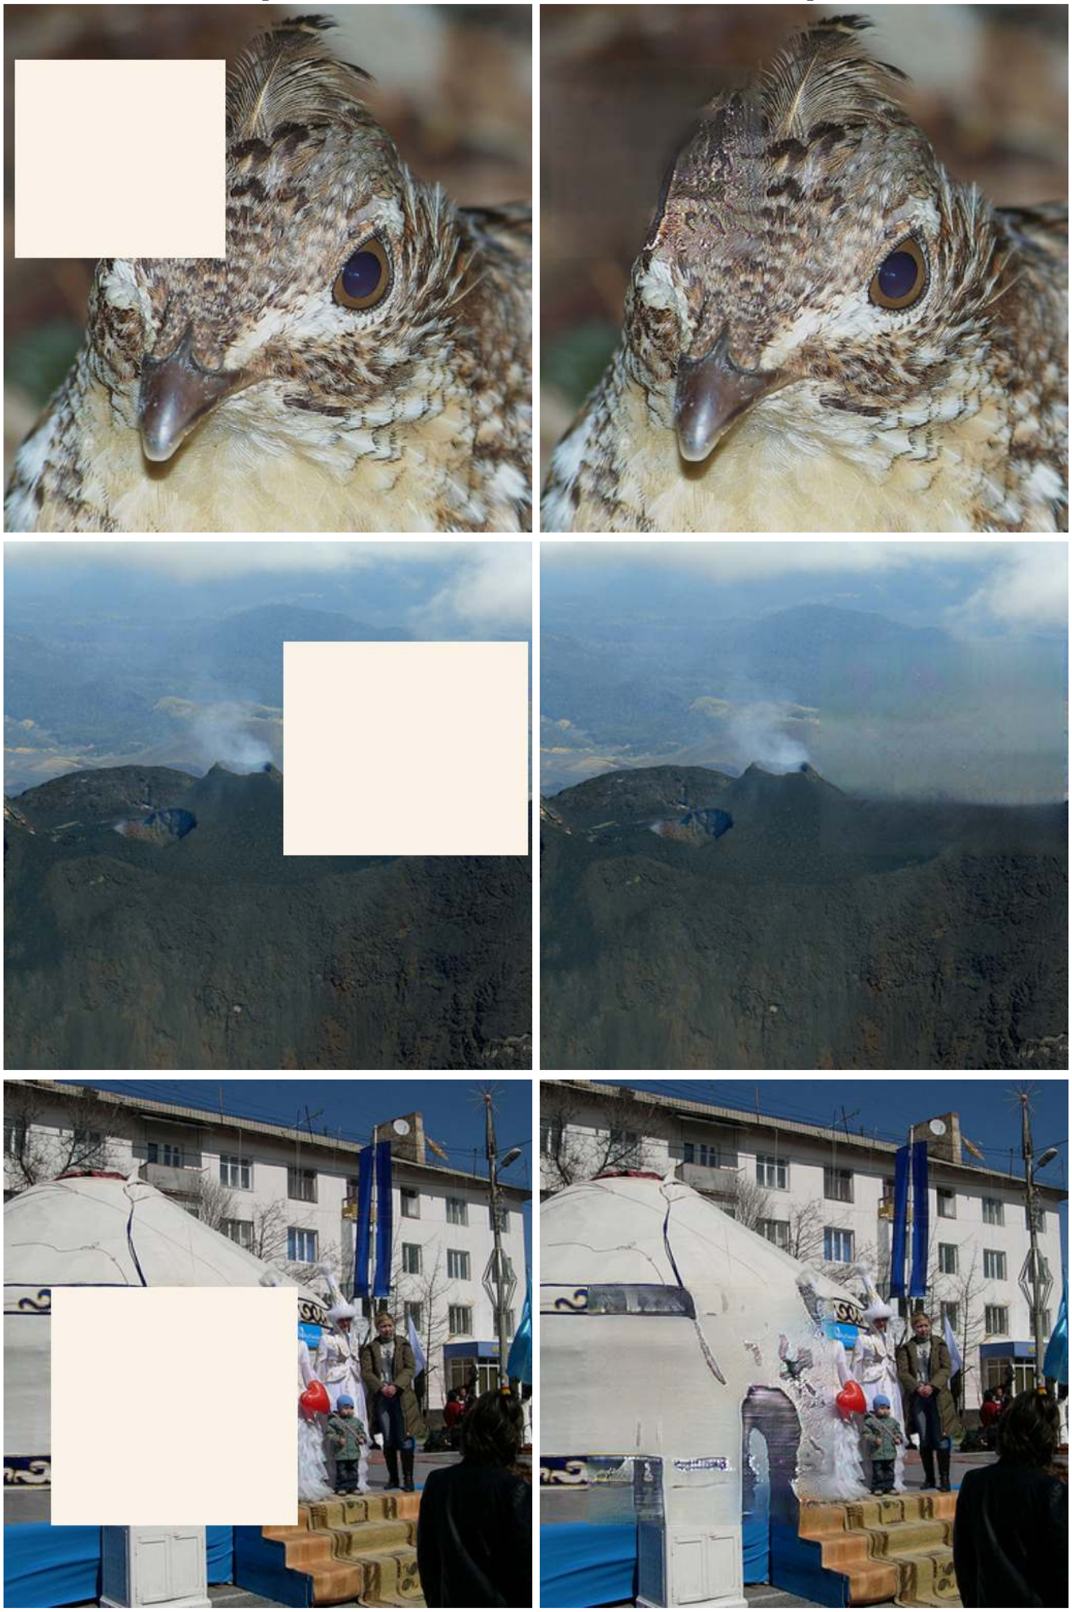

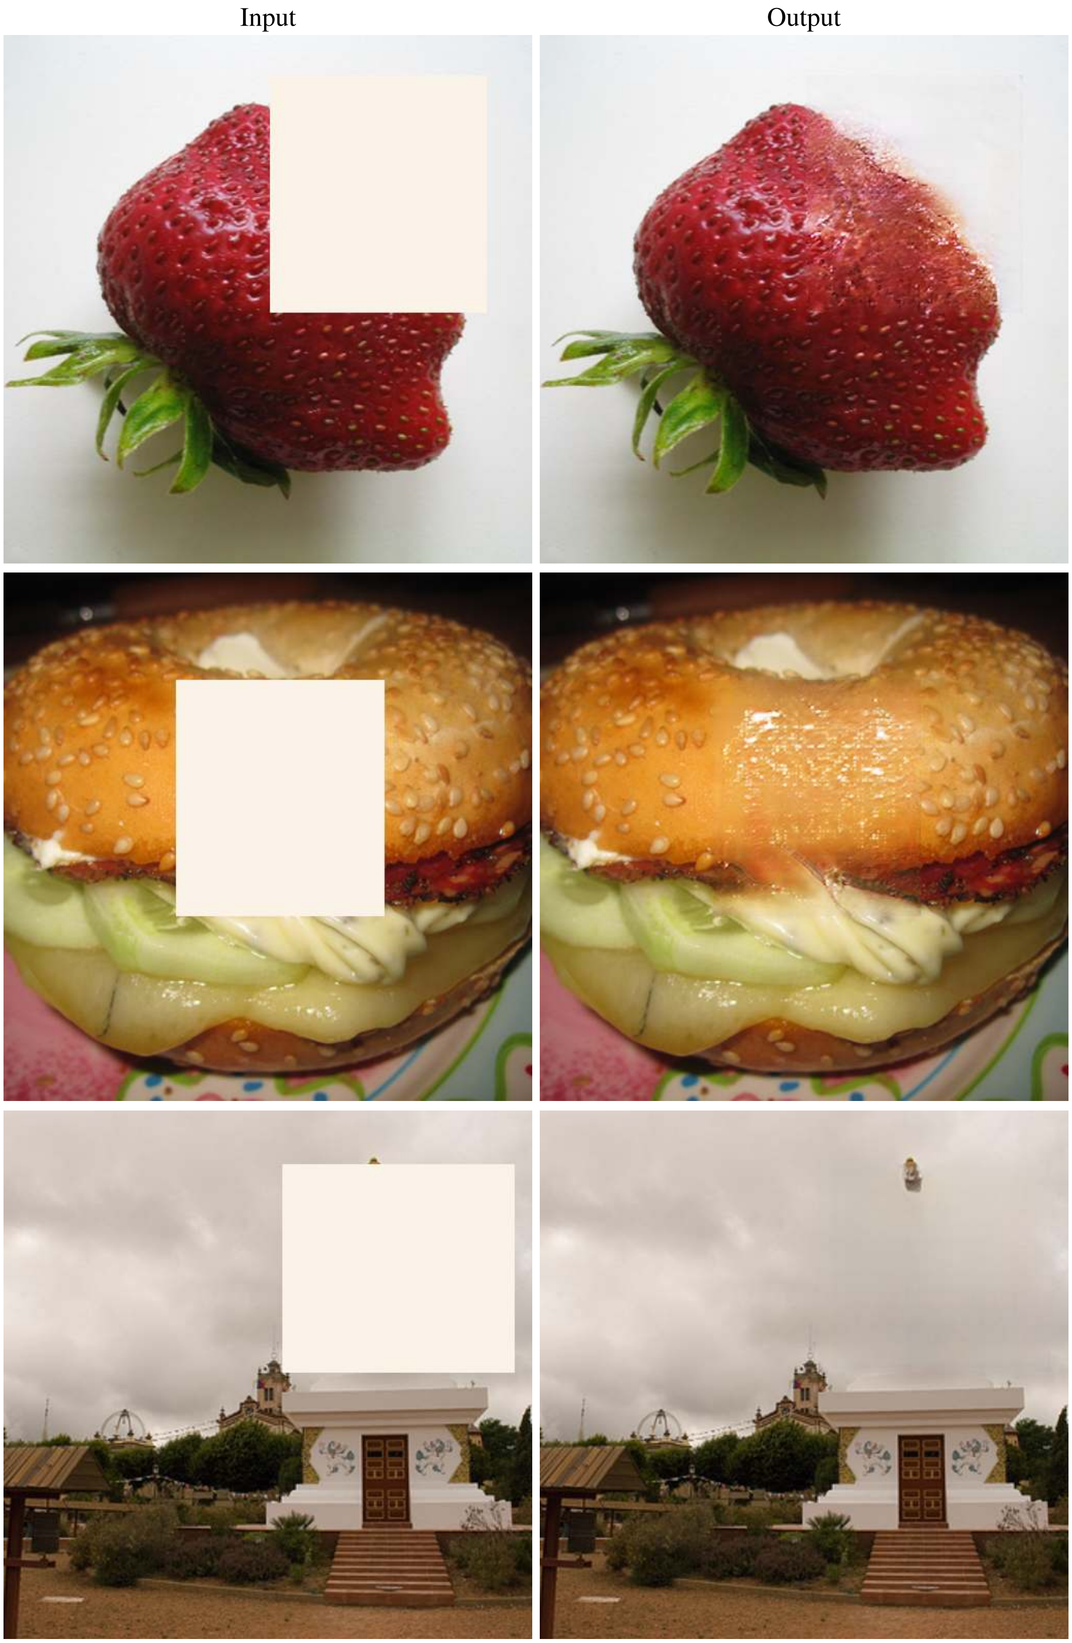
Input
Output

Input Output

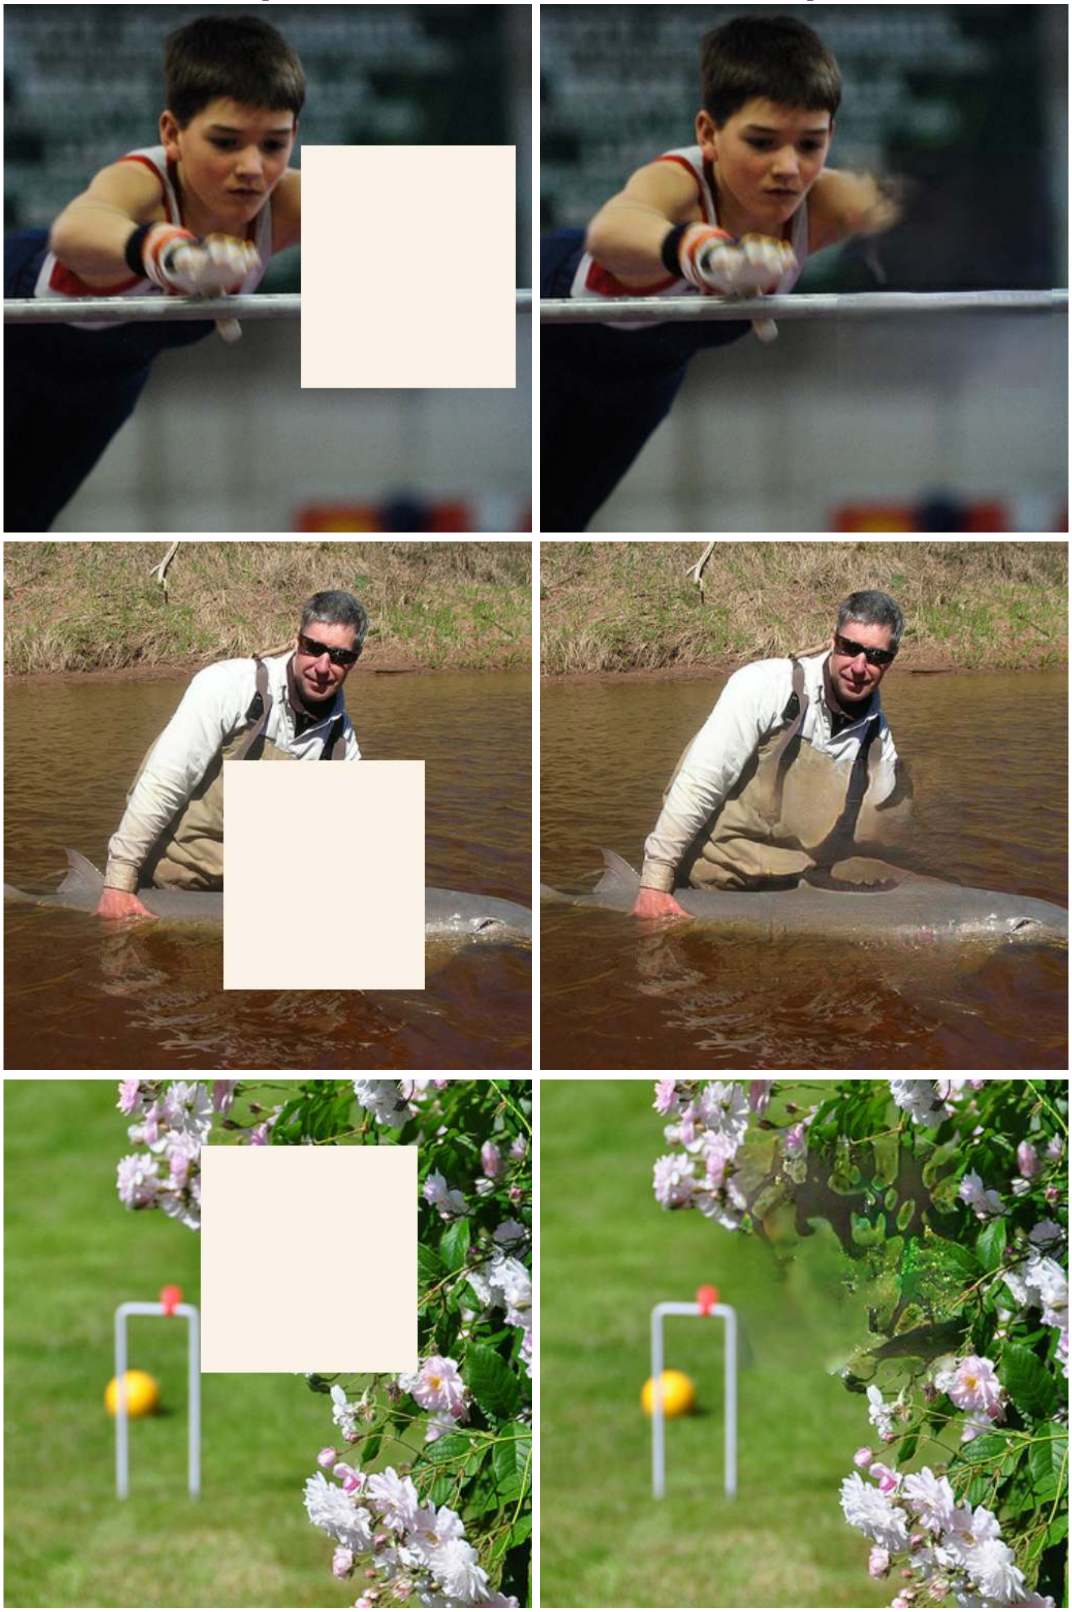

Input Output

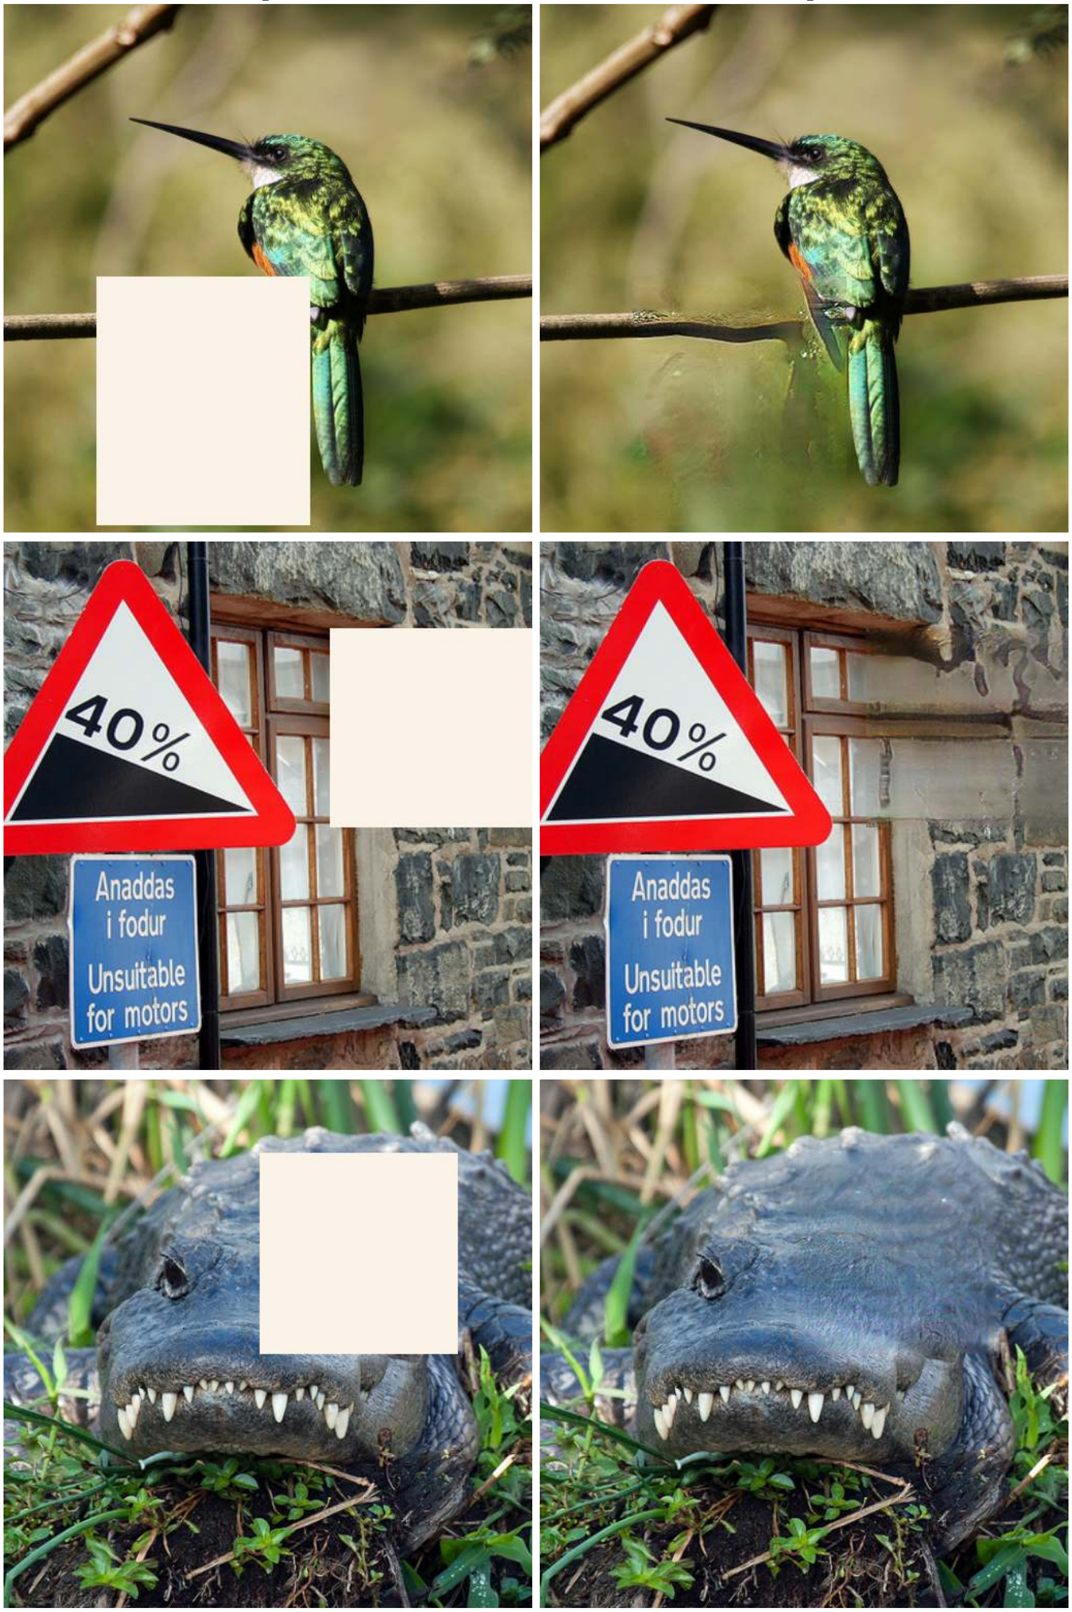

## 1.2. Google Street View

Images from the Google Street View dataset are scaled to 256x256. 128x128 sized center patches are extracted from inputs. Our network reconstructs whole images without using the mask location.

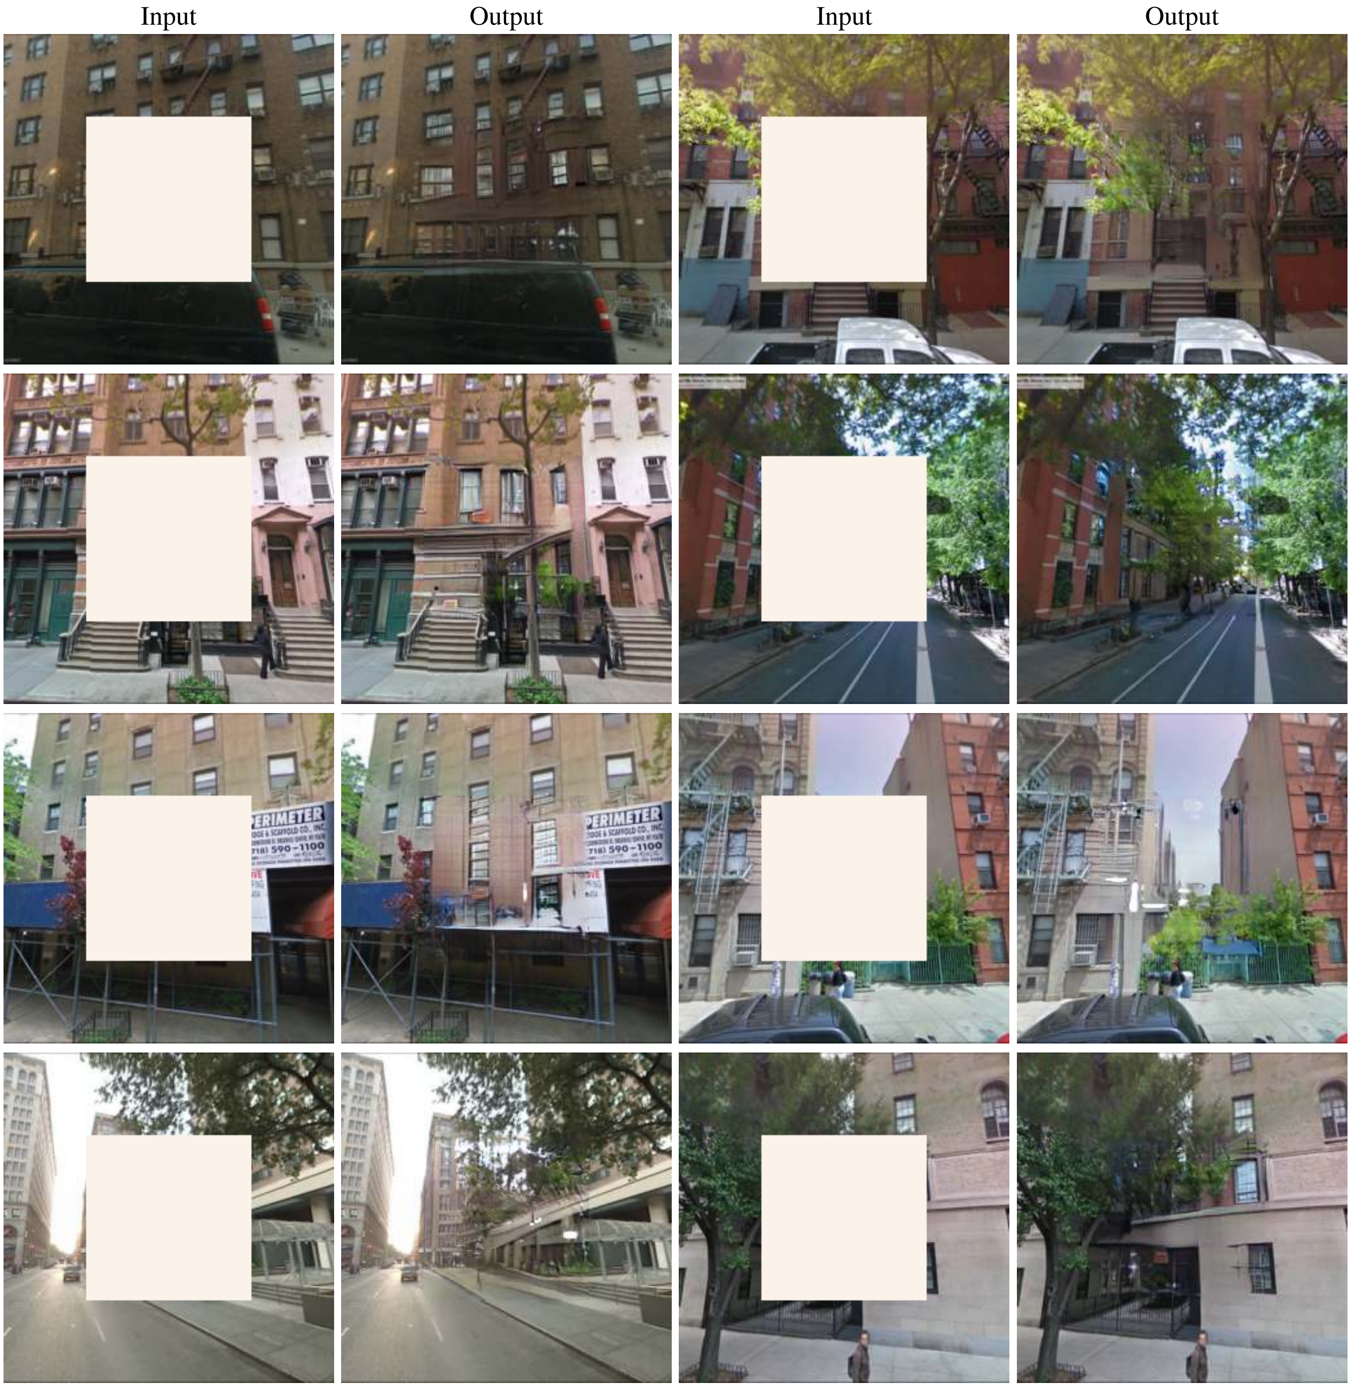

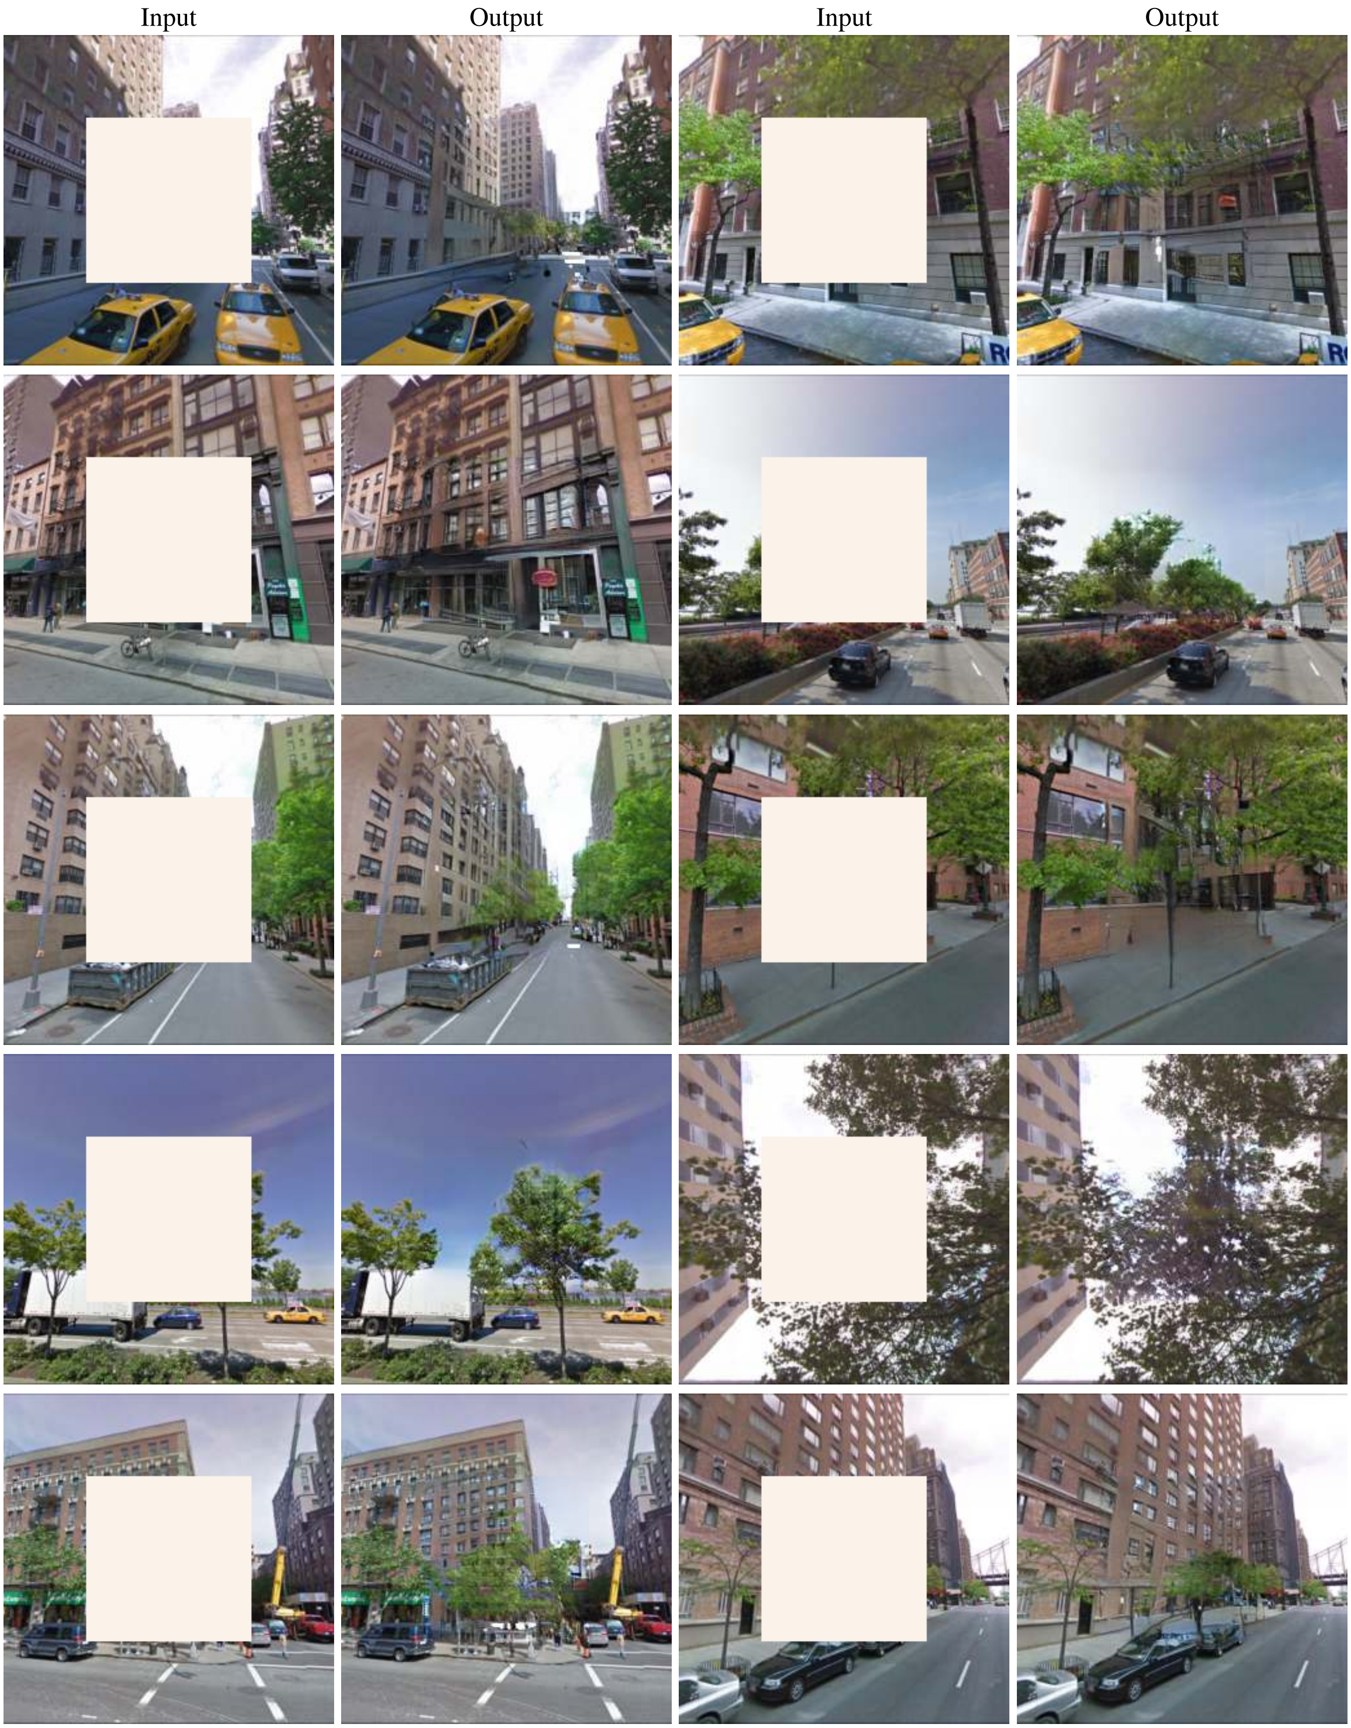
Input
Output
Input
Output

Input Output Input Output

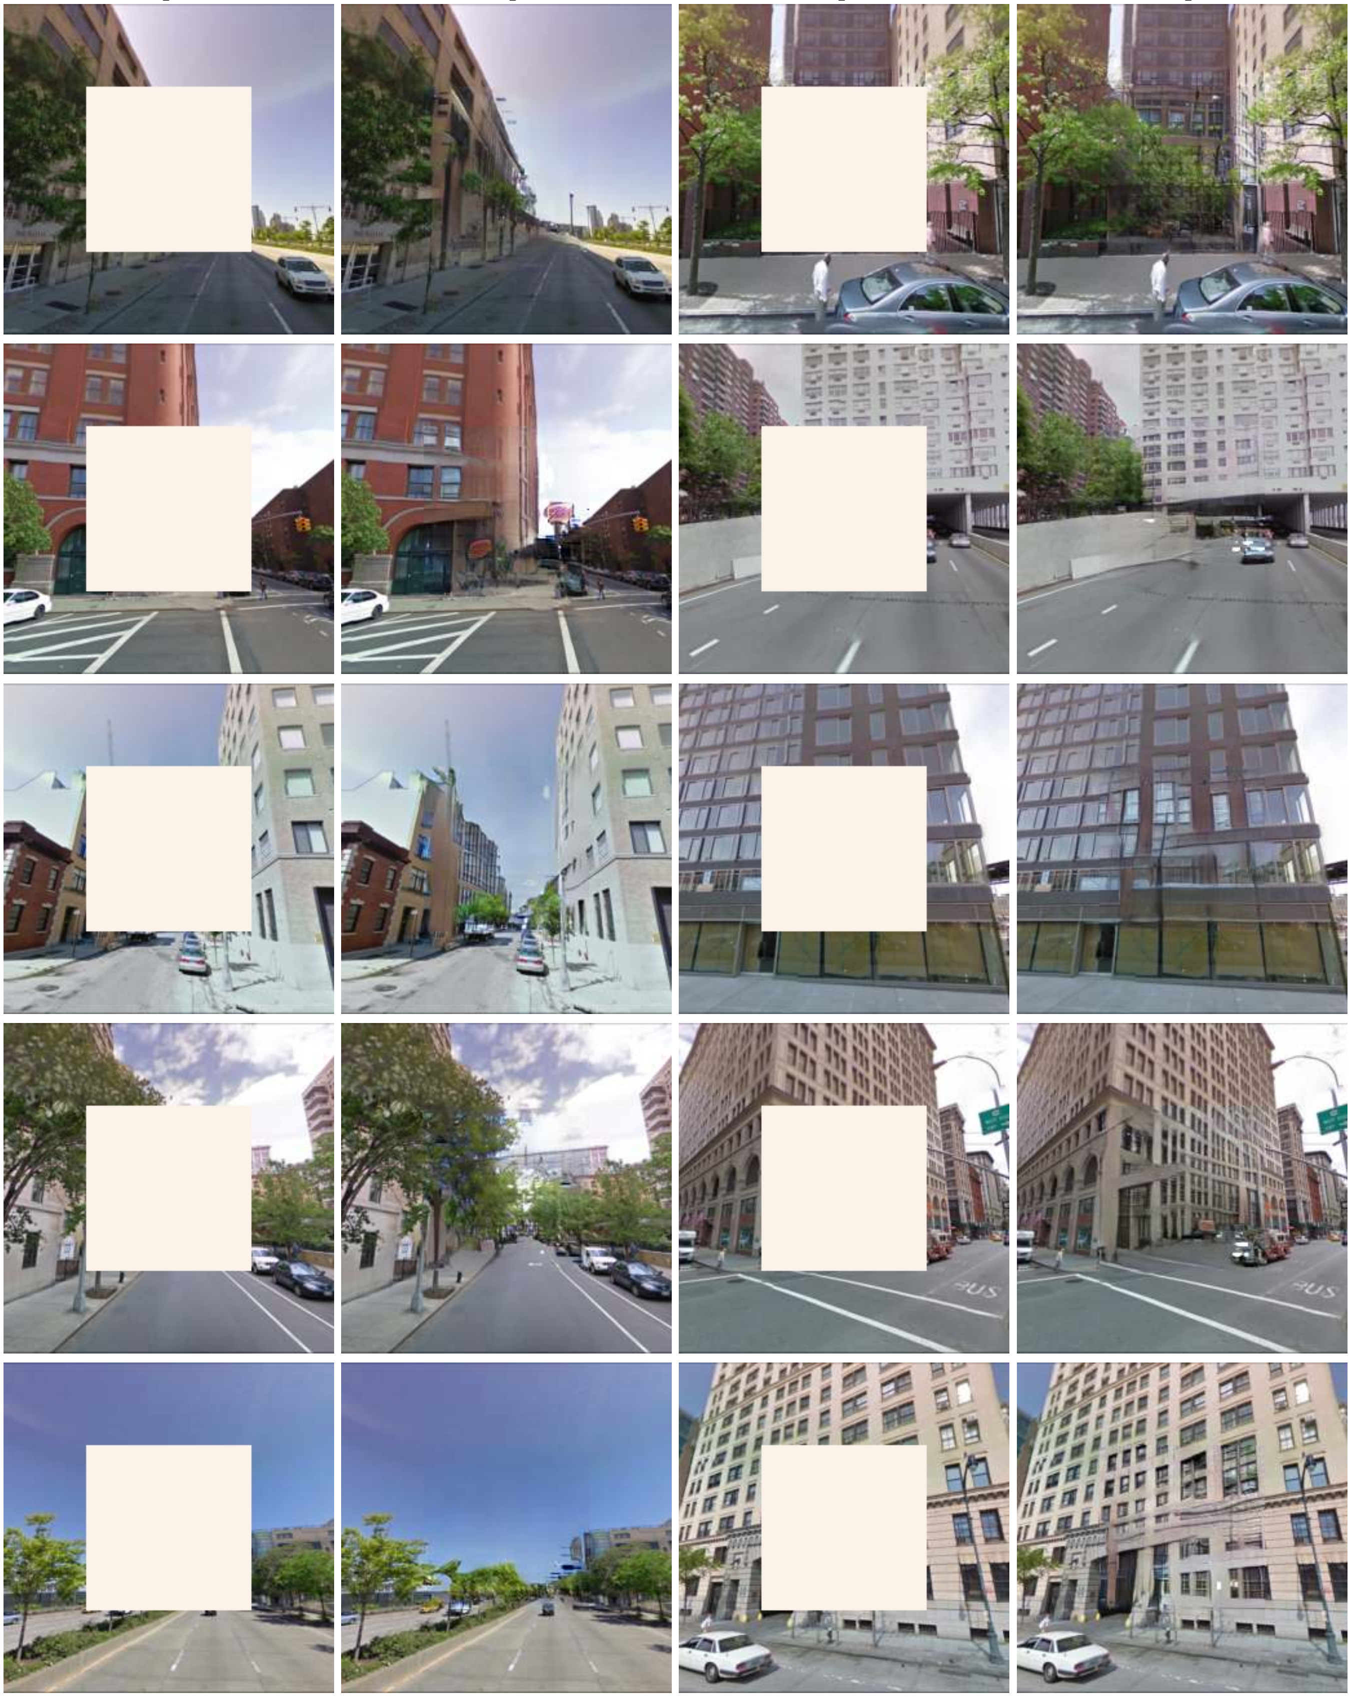

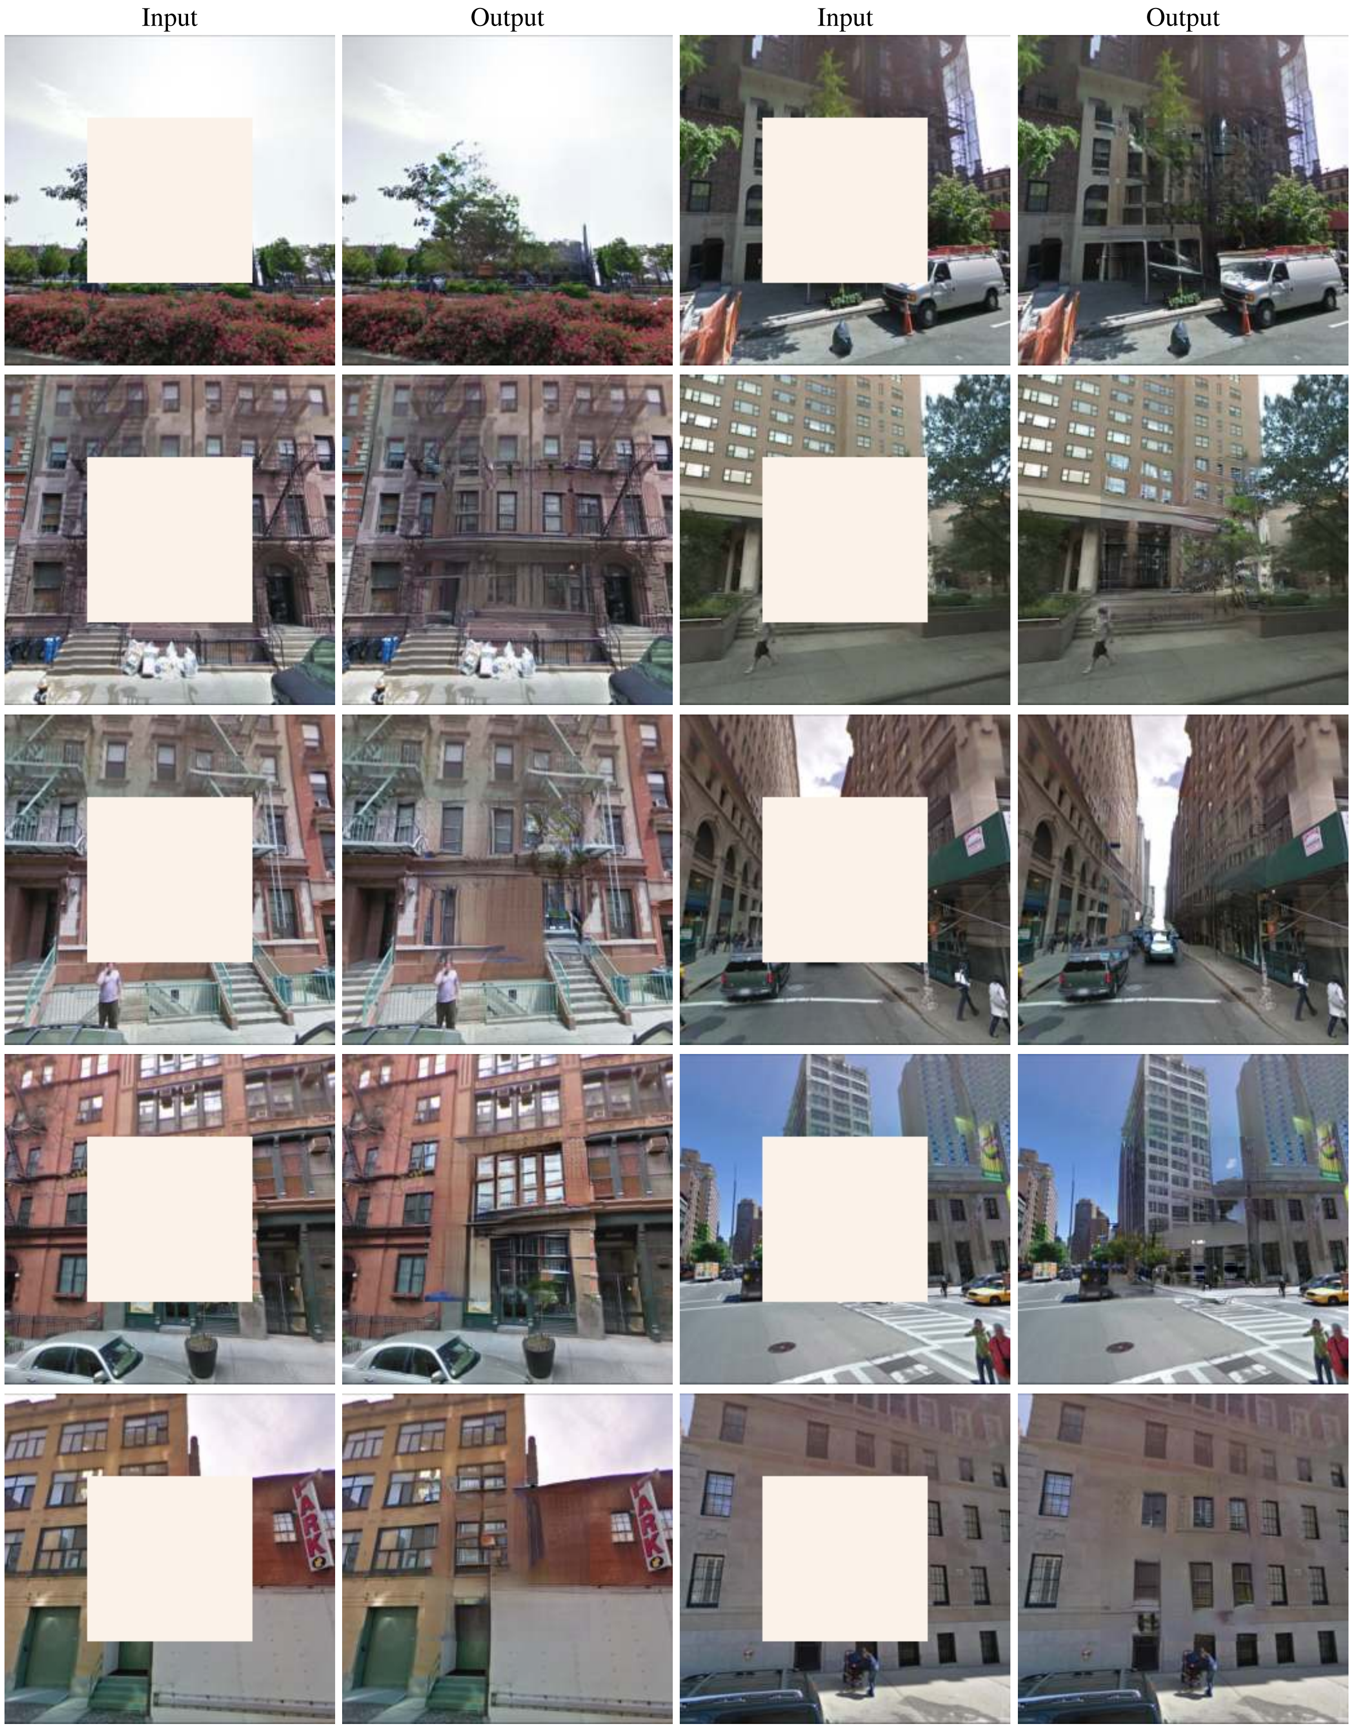
Input
Output
Input
Output

Input Output Input Output

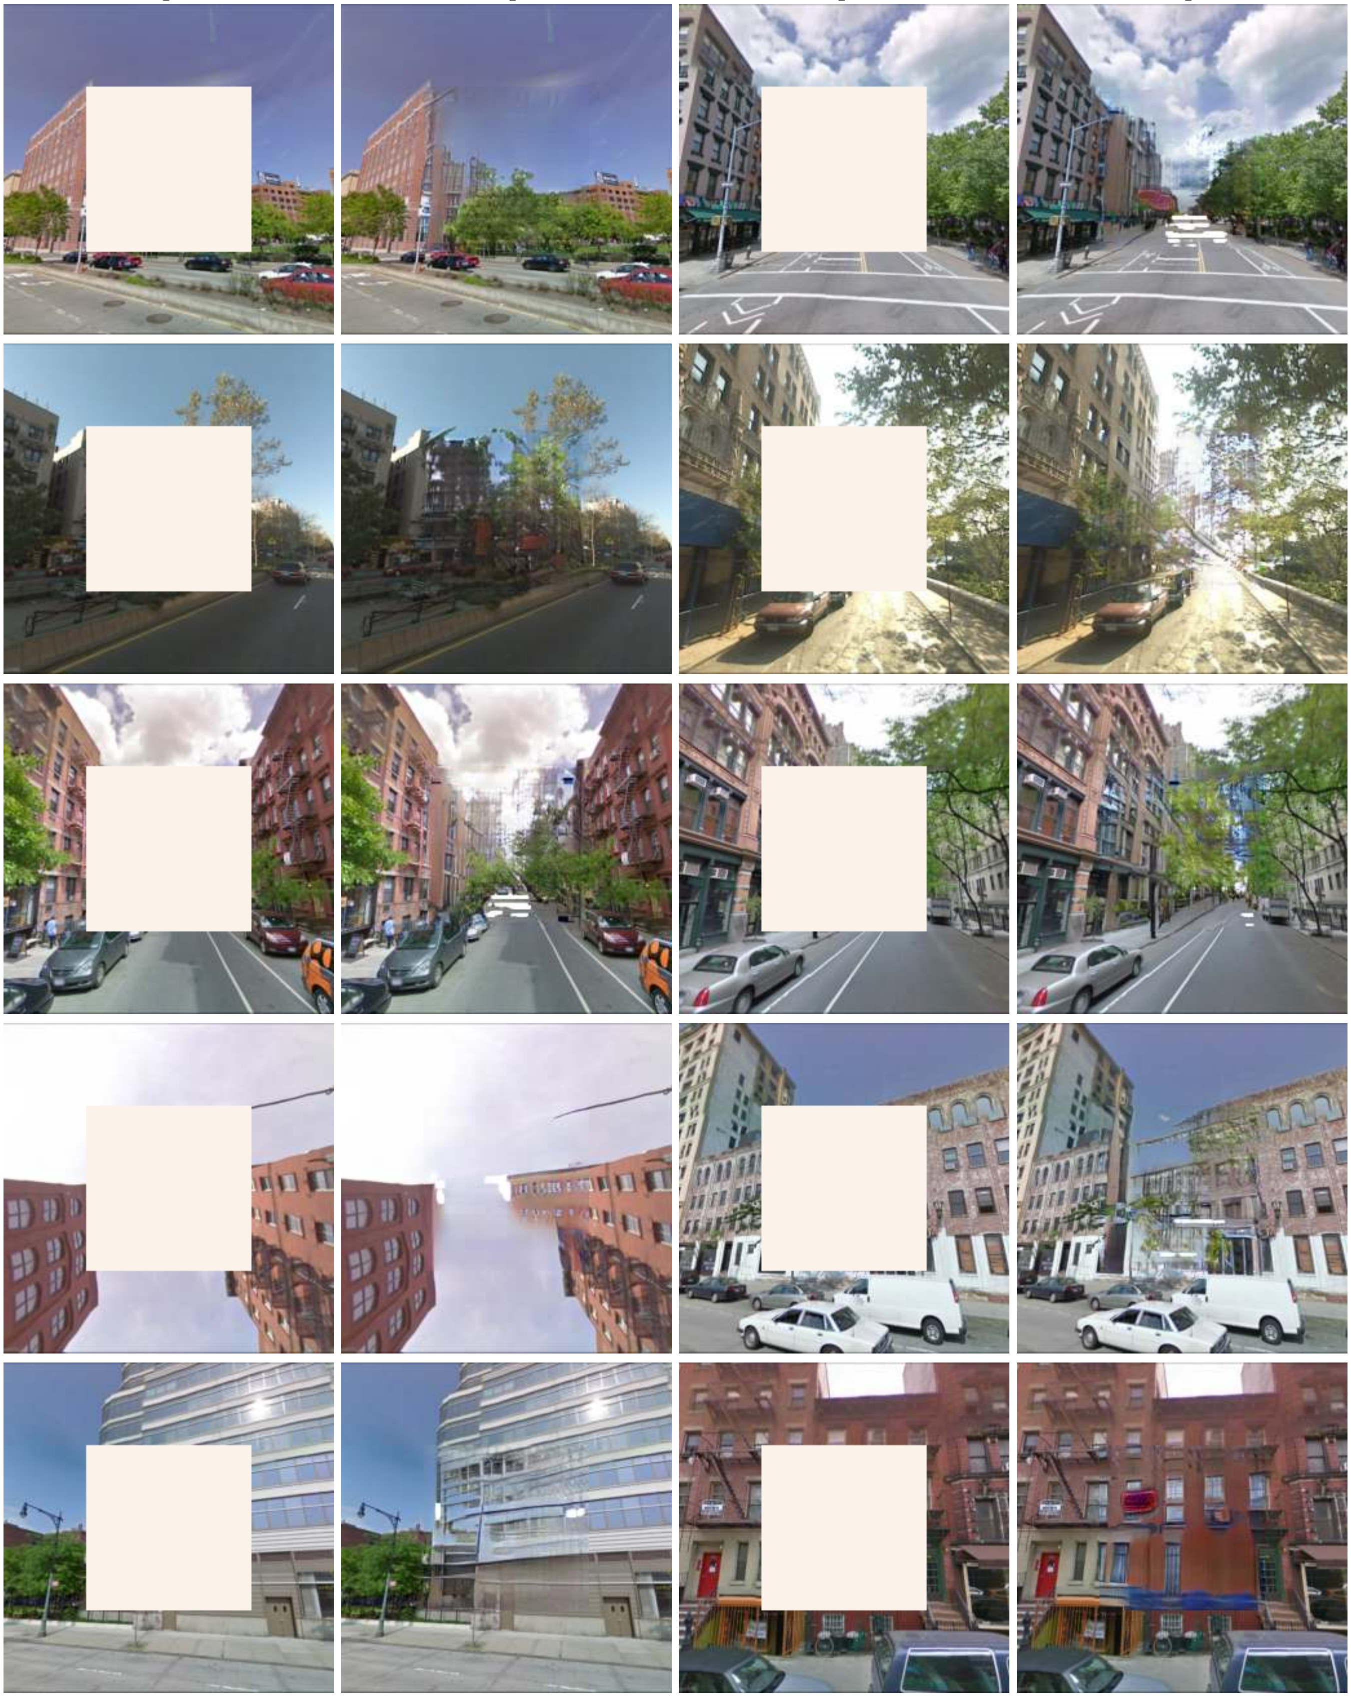

### 1.3. Places2

We train PGGAN with 8 millions images from Places2 dataset. During the training, inputs are scaled to size of 256x256 and random sized mask is applied to them. Results are presented below.

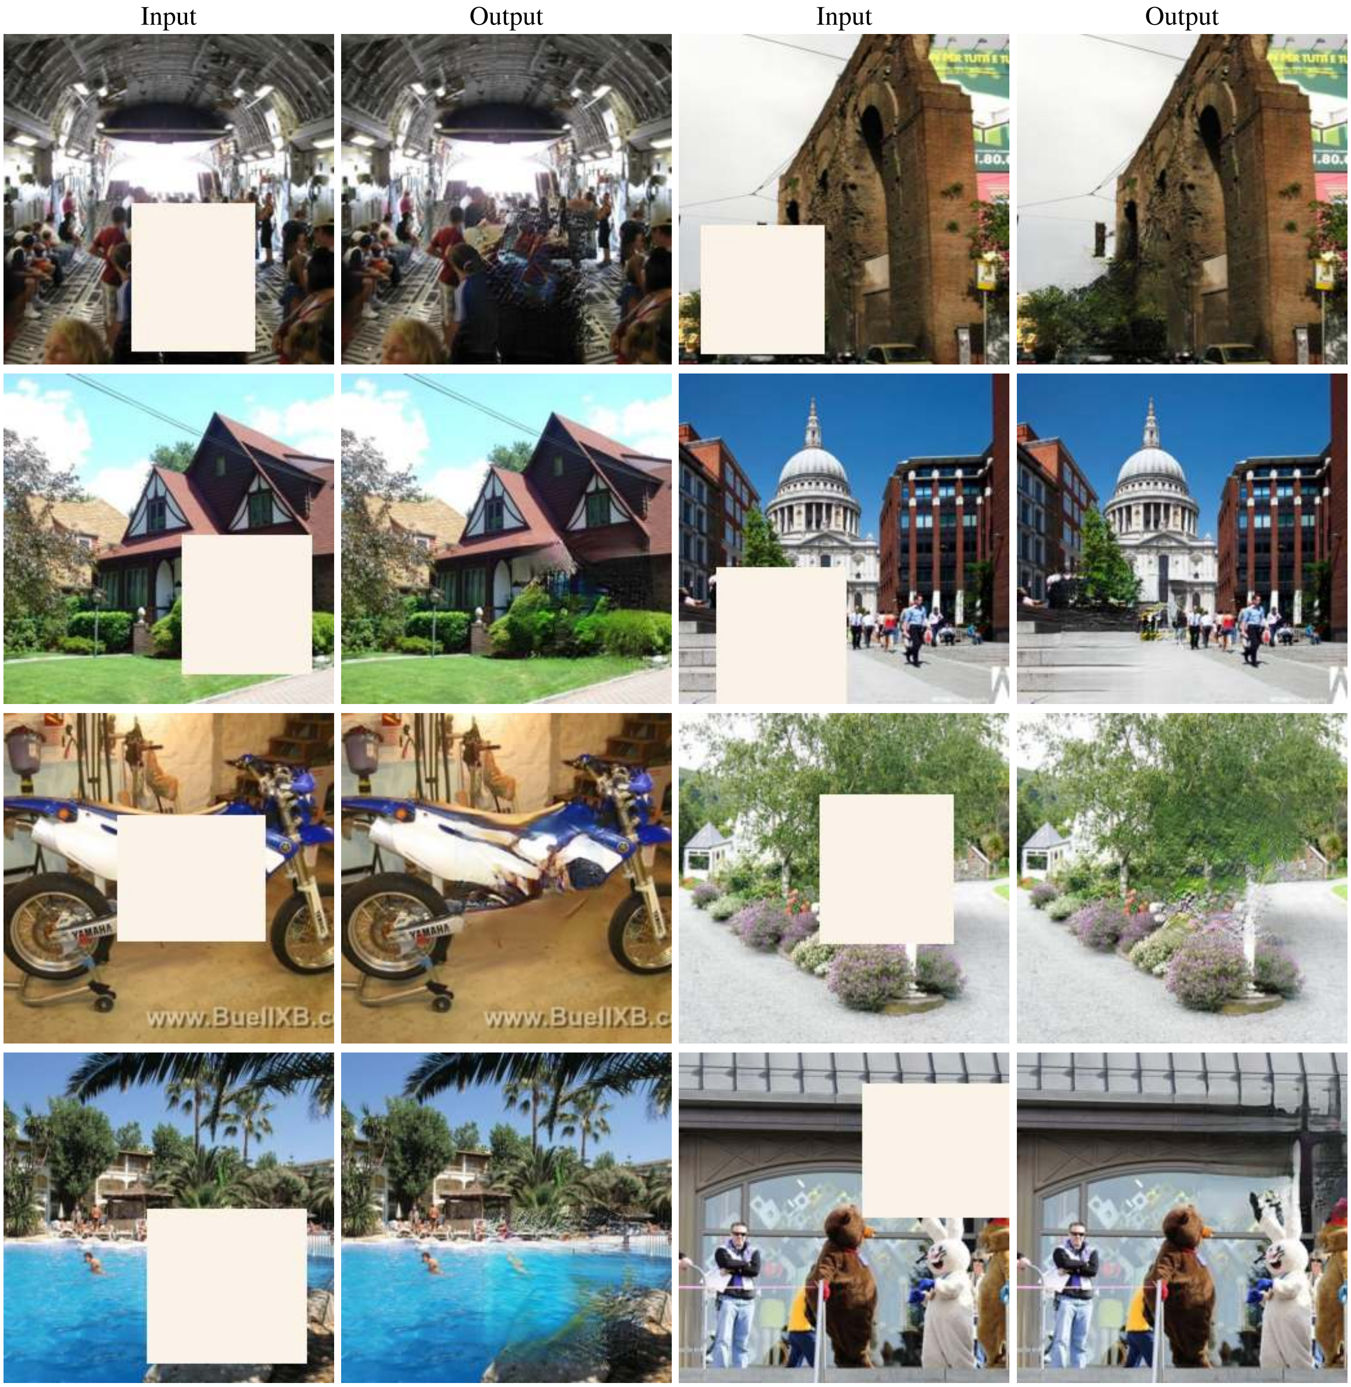

Input Output Input Output

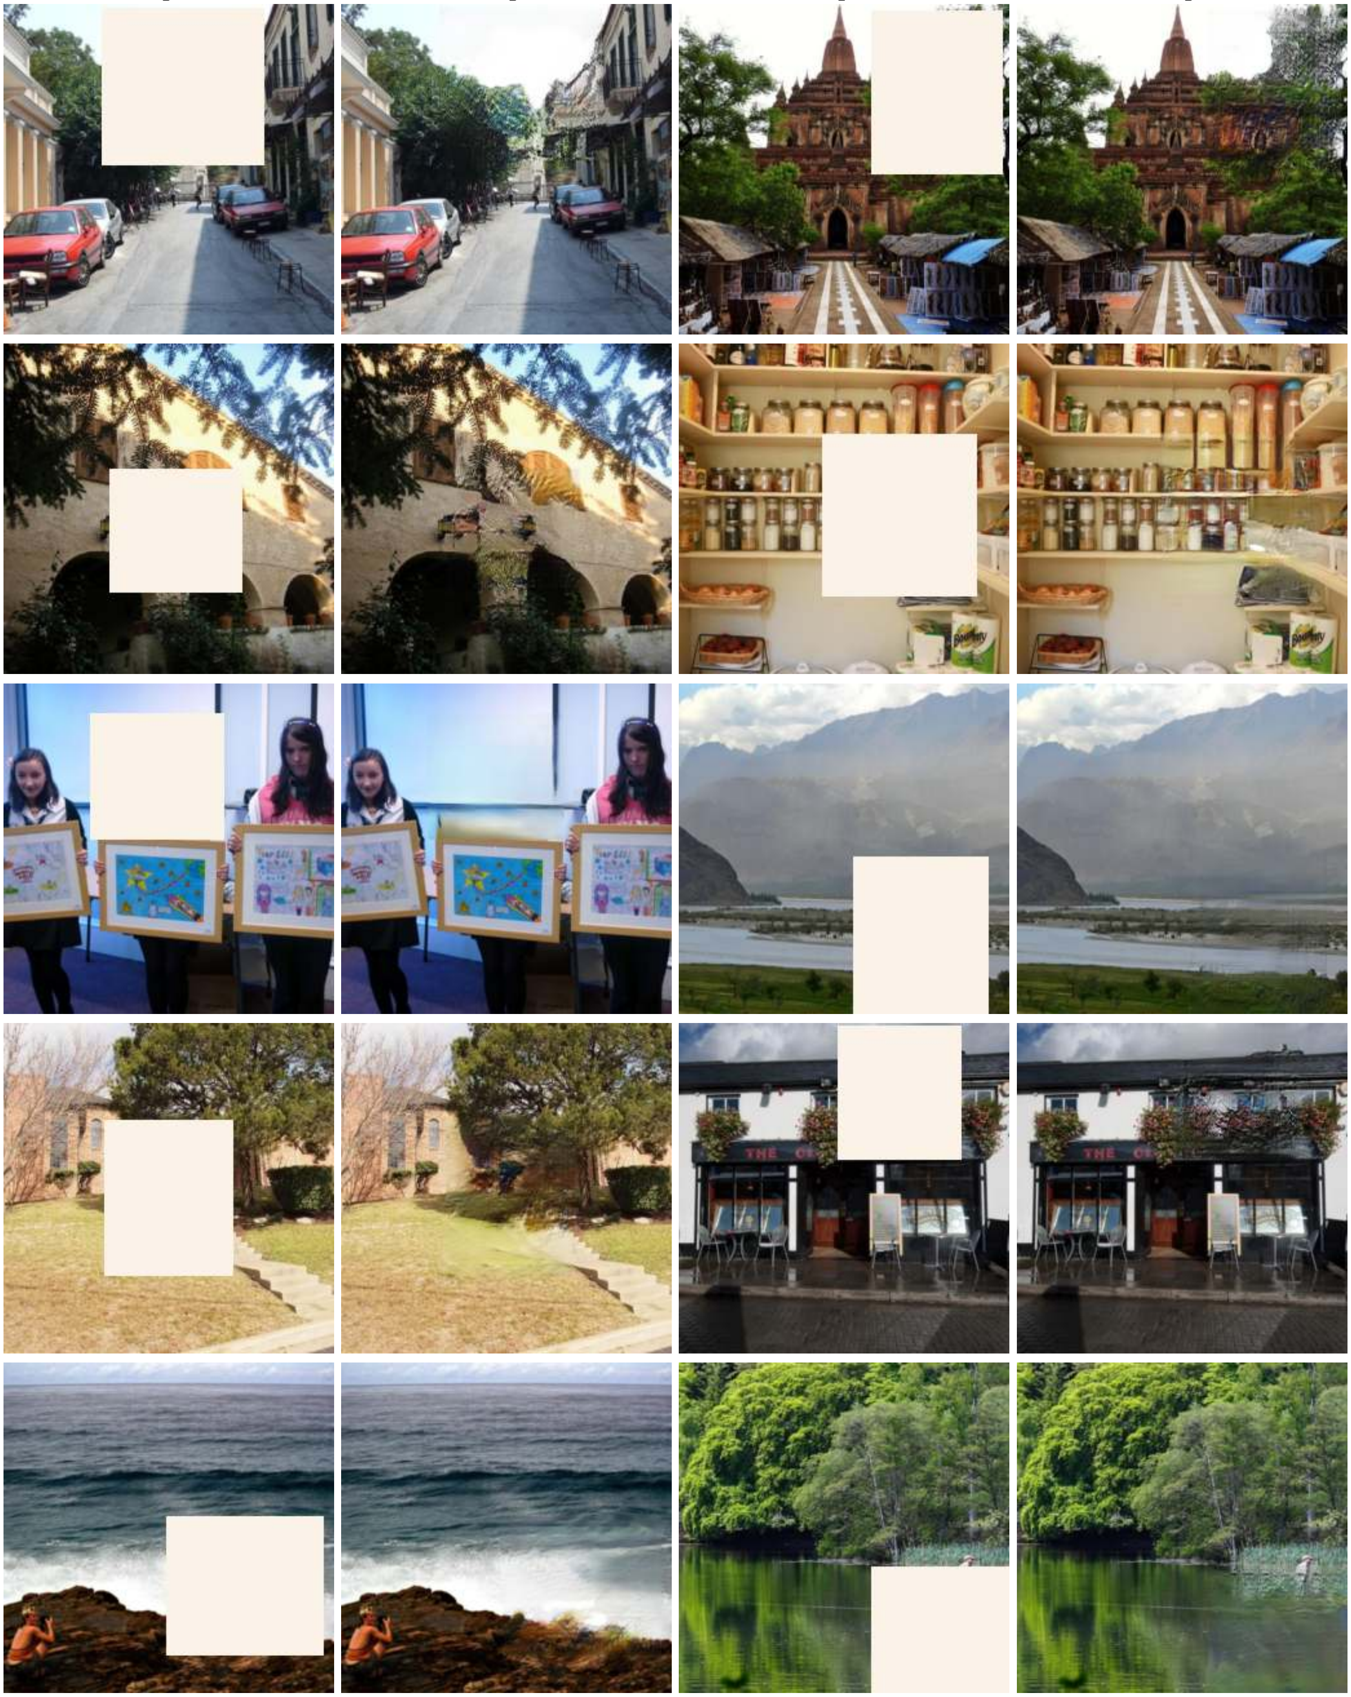

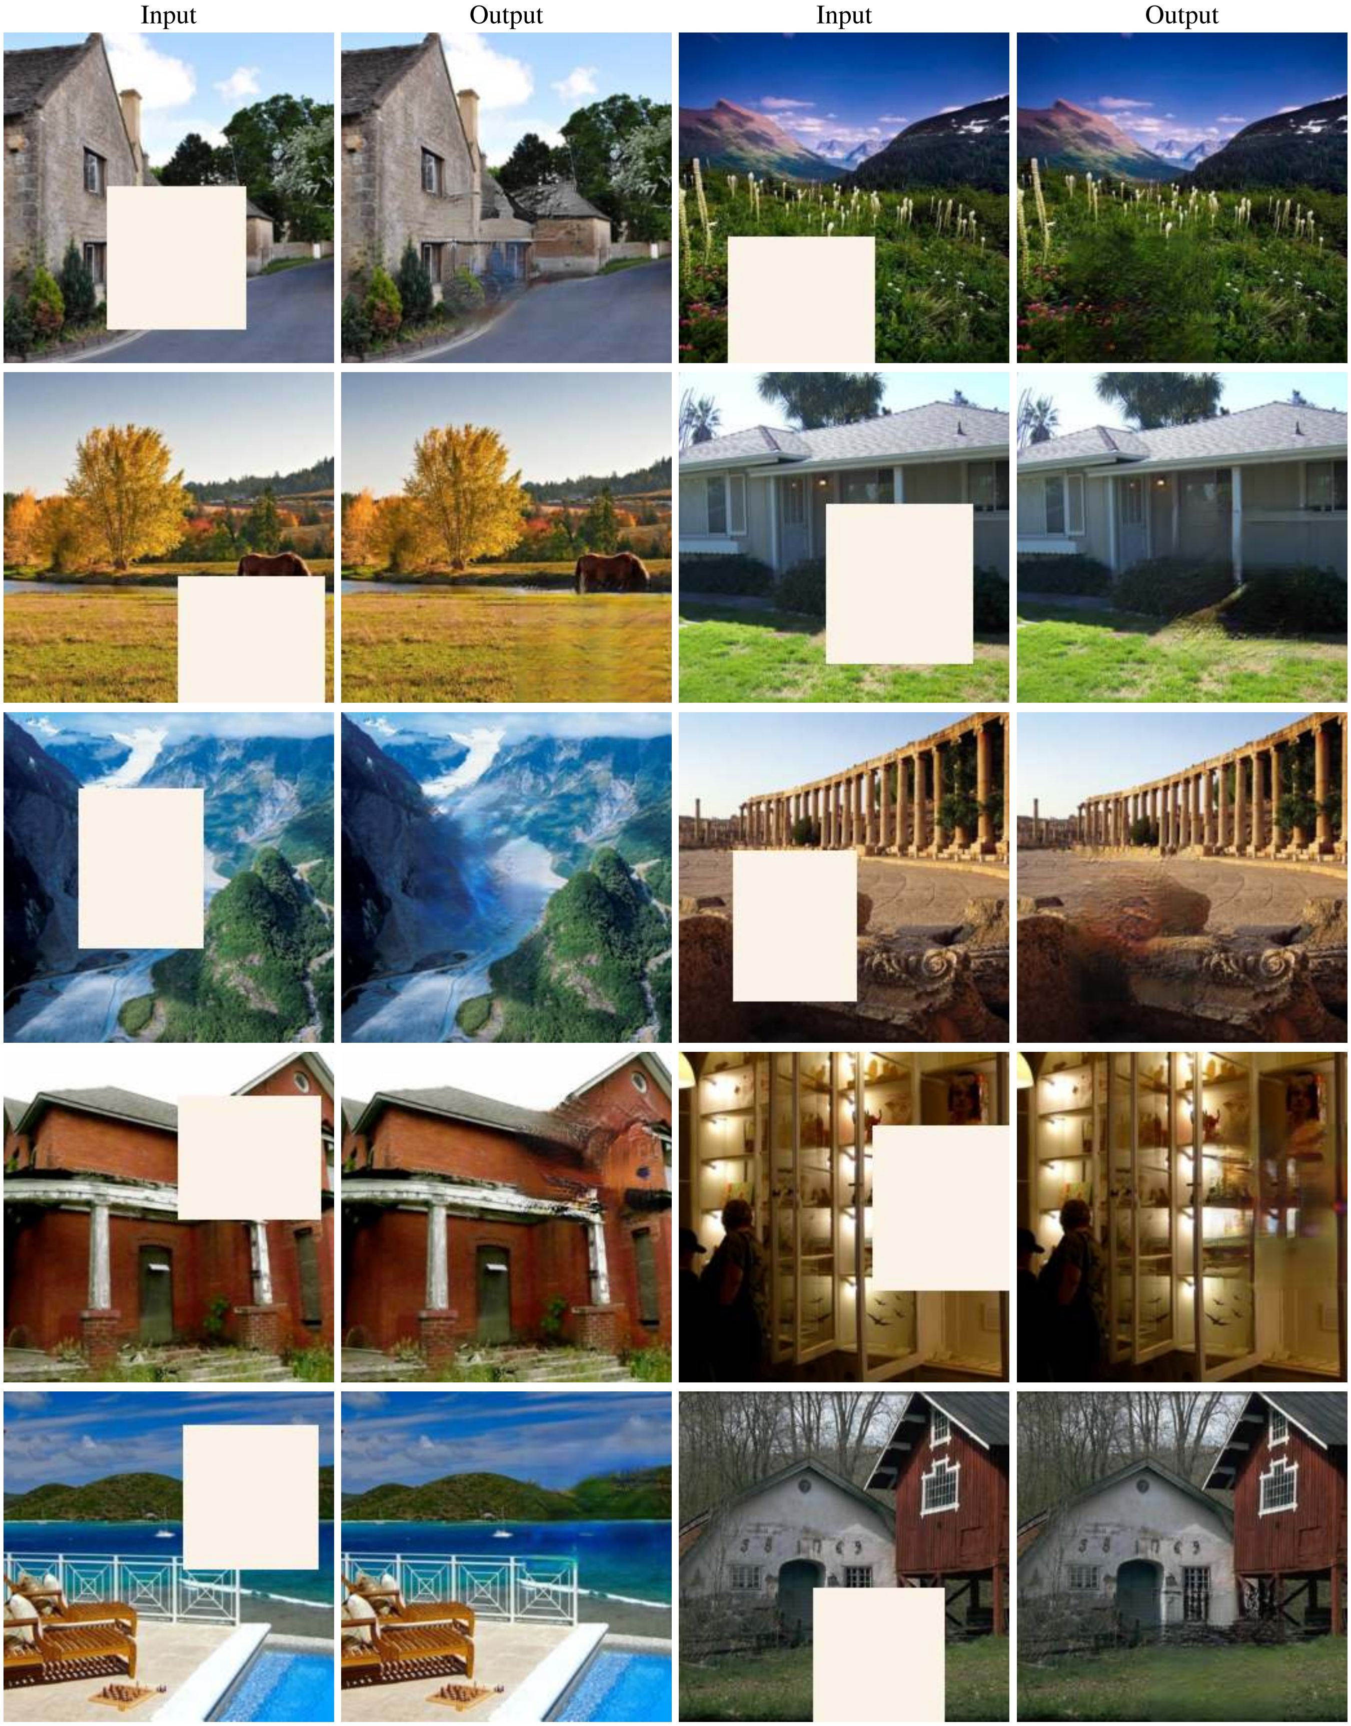
Input
Output
Input
Output

Input Output Input Output

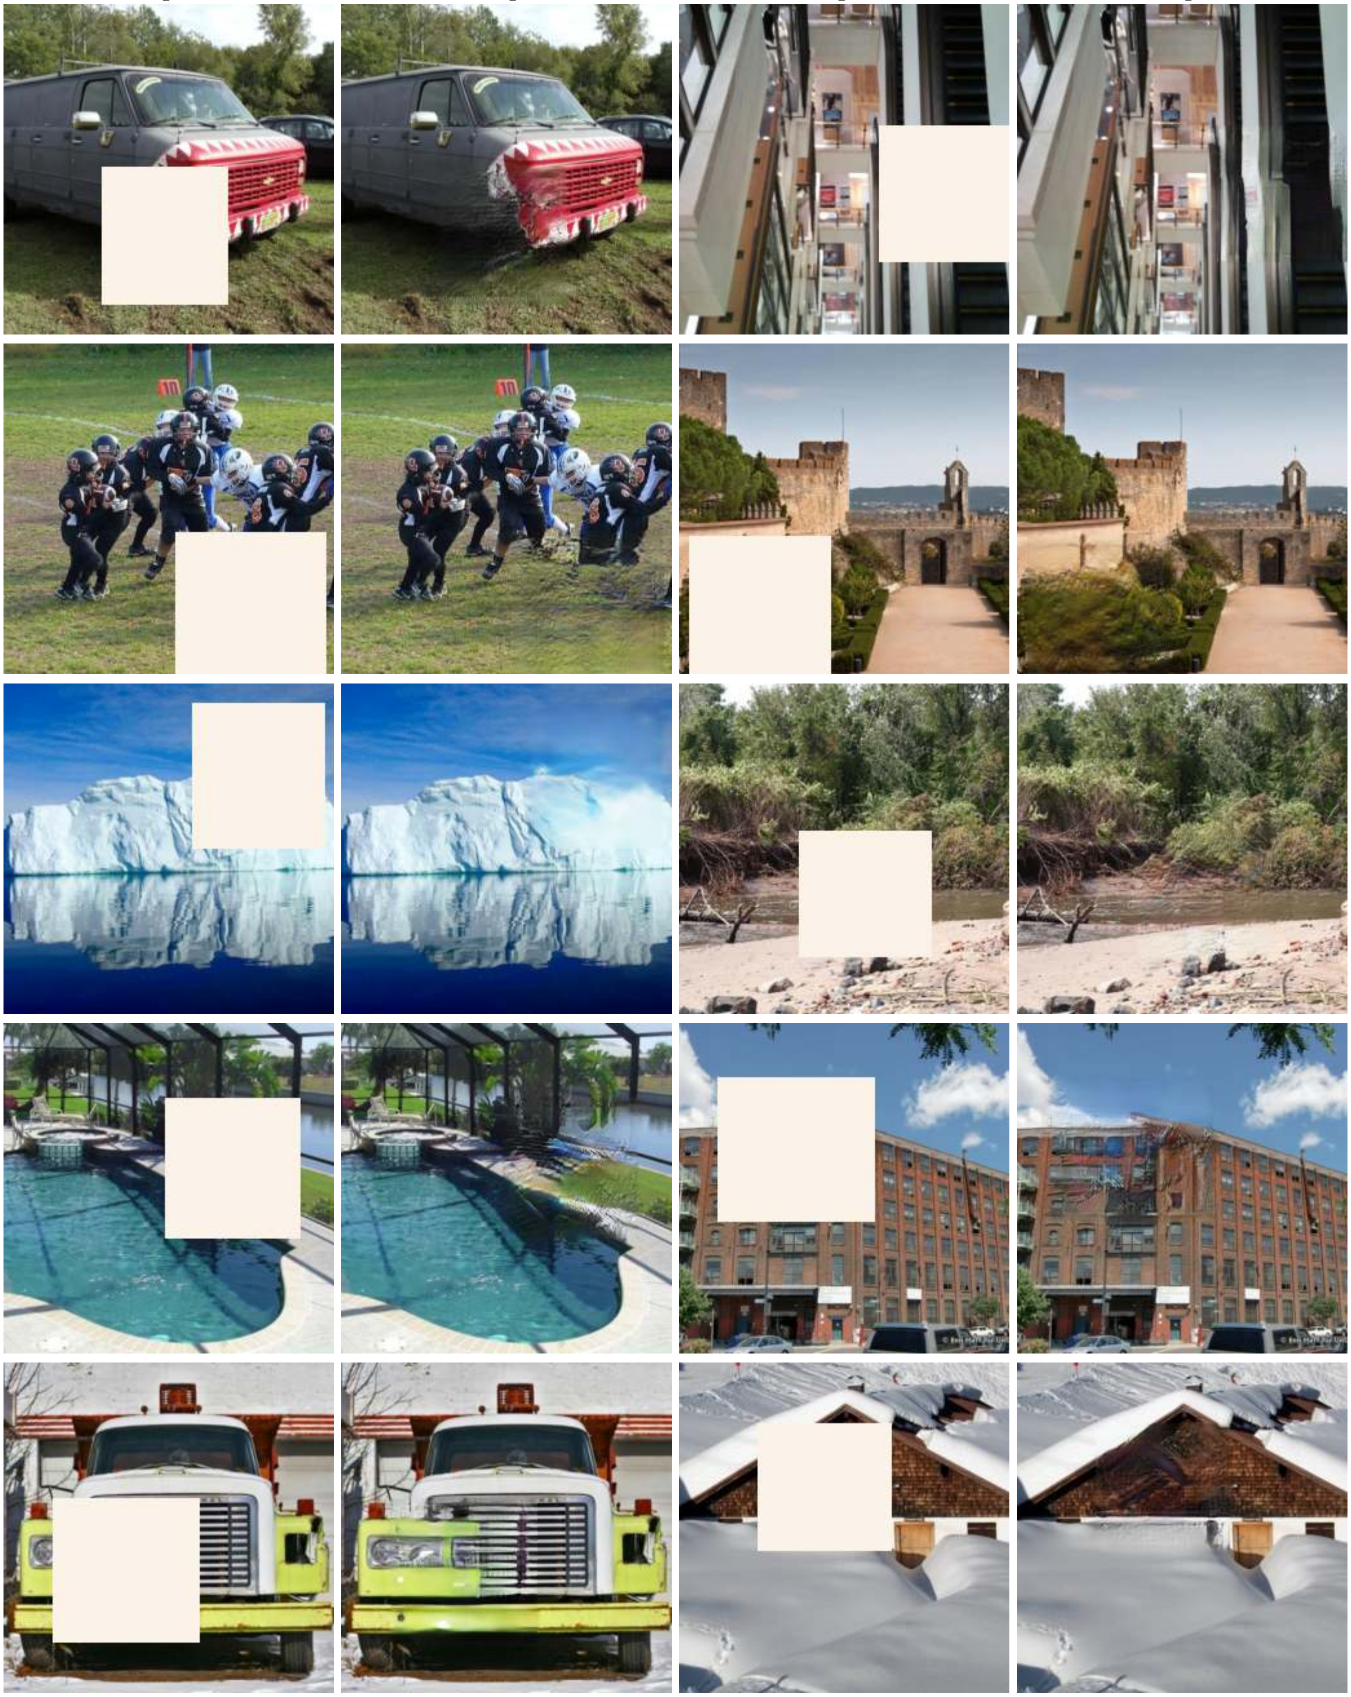

Supplement: Supplementary file 1 [file supp.pdf]
